# Supplementary material for: Safe Inference-Time Alignment via Lagrangian Reward Augmentation
Source: arXiv:2607.02781 source file (2026-11-25)
Supplement: Supplementary file 1 [file appendix.tex]

\section{Dual}

\begin{proposition}[Dual reduction of KL-regularized safe alignment]
\label{prop:primal-safe}
Let $D_x$ be a distribution over prompts $x$, let $\pi_{\mathrm{ref}}(\cdot \mid x)$ be a reference policy,
and let $r,c$ be measurable reward and cost functions such that, for every $x$ and $\lambda \ge 0$,
\[
\mathbb{E}_{y \sim \pi_{\mathrm{ref}}(\cdot \mid x)}
\!\left[\exp\!\left(\frac{r(x,y)-\lambda c(x,y)}{\beta}\right)\right] < \infty.
\]
Consider the optimization problem
\begin{equation}
\sup_{\pi}
\;
\mathbb{E}_{x \sim D_x}\!\left[
\mathbb{E}_{y \sim \pi(\cdot \mid x)} r(x,y)
-\beta D_{\mathrm{KL}}\!\left(\pi(\cdot \mid x)\,\|\,\pi_{\mathrm{ref}}(\cdot \mid x)\right)
\right]
\quad
\text{s.t.}
\quad
\mathbb{E}_{x \sim D_x}\mathbb{E}_{y \sim \pi(\cdot \mid x)} c(x,y) \le \tau,
\label{eq:primal-safe}
\end{equation}
where the supremum is over all conditional distributions $\pi(\cdot\mid x)$ absolutely continuous
with respect to $\pi_{\mathrm{ref}}(\cdot\mid x)$.

For $\lambda \ge 0$, define the net reward
\[
r_\lambda(x,y) := r(x,y)-\lambda c(x,y),
\]
and the dual function
\[
g(\lambda)
:=
\sup_{\pi}
\mathbb{E}_{x \sim D_x}\!\left[
\mathbb{E}_{y \sim \pi(\cdot \mid x)} r_\lambda(x,y)
-\beta D_{\mathrm{KL}}\!\left(\pi(\cdot \mid x)\,\|\,\pi_{\mathrm{ref}}(\cdot \mid x)\right)
\right]
+\lambda \tau.
\]
Then, for every $\lambda \ge 0$, the inner supremum is attained by
\begin{equation}
\pi_\lambda^*(y\mid x)
=
\frac{\pi_{\mathrm{ref}}(y\mid x)\exp\!\left(r_\lambda(x,y)/\beta\right)}
{\mathbb{E}_{y' \sim \pi_{\mathrm{ref}}(\cdot\mid x)}
\left[\exp\!\left(r_\lambda(x,y')/\beta\right)\right]},
\label{eq:gibbs-policy}
\end{equation}
and the dual objective admits the closed form
\begin{equation}
g(\lambda)
=
\beta \,
\mathbb{E}_{x \sim D_x}
\log
\mathbb{E}_{y \sim \pi_{\mathrm{ref}}(\cdot \mid x)}
\left[
\exp\!\left(\frac{r(x,y)-\lambda c(x,y)}{\beta}\right)
\right]
+\lambda \tau.
\label{eq:dual-closed-form}
\end{equation}
Consequently, the dual problem is the one-dimensional convex optimization problem
\[
\inf_{\lambda \ge 0} g(\lambda).
\]
\end{proposition}

\begin{proof}
For fixed $\lambda \ge 0$, the Lagrangian is
\[
\mathcal{L}(\pi,\lambda)
=
\mathbb{E}_{x \sim D_x}\!\left[
\mathbb{E}_{y \sim \pi(\cdot \mid x)} r_\lambda(x,y)
-\beta D_{\mathrm{KL}}\!\left(\pi(\cdot \mid x)\,\|\,\pi_{\mathrm{ref}}(\cdot \mid x)\right)
\right]
+\lambda \tau.
\]
Since the objective is separable in $x$, it suffices to solve, for each fixed $x$,
\[
\sup_{q}
\left\{
\mathbb{E}_{y \sim q} r_\lambda(x,y)
-\beta D_{\mathrm{KL}}\!\left(q\,\|\,\pi_{\mathrm{ref}}(\cdot \mid x)\right)
\right\},
\]
where the supremum is over distributions $q$ absolutely continuous with respect to
$\pi_{\mathrm{ref}}(\cdot\mid x)$.

Define
\[
Z_\lambda(x)
:=
\mathbb{E}_{y \sim \pi_{\mathrm{ref}}(\cdot \mid x)}
\left[
\exp\!\left(\frac{r_\lambda(x,y)}{\beta}\right)
\right],
\]
and
\[
\pi_\lambda^*(y\mid x)
:=
\frac{\pi_{\mathrm{ref}}(y\mid x)\exp\!\left(r_\lambda(x,y)/\beta\right)}{Z_\lambda(x)}.
\]
Then, for any admissible $q$,
\begin{align*}
D_{\mathrm{KL}}(q \,\|\, \pi_\lambda^*(\cdot\mid x))
&=
\mathbb{E}_{y \sim q}
\left[
\log \frac{q(y)}{\pi_\lambda^*(y\mid x)}
\right] \\
&=
D_{\mathrm{KL}}(q \,\|\, \pi_{\mathrm{ref}}(\cdot\mid x))
-\frac{1}{\beta}\mathbb{E}_{y \sim q}[r_\lambda(x,y)]
+\log Z_\lambda(x).
\end{align*}
Rearranging yields
\[
\mathbb{E}_{y \sim q}[r_\lambda(x,y)]
-\beta D_{\mathrm{KL}}(q \,\|\, \pi_{\mathrm{ref}}(\cdot\mid x))
=
\beta \log Z_\lambda(x)
-\beta D_{\mathrm{KL}}(q \,\|\, \pi_\lambda^*(\cdot\mid x)).
\]
Since the KL divergence is nonnegative, the supremum is attained at $q=\pi_\lambda^*(\cdot\mid x)$,
and the optimal value is $\beta \log Z_\lambda(x)$. Taking expectation over $x$ proves
\eqref{eq:dual-closed-form}.
\end{proof}

\begin{corollary}[Gradient and convexity of the dual objective]
Let $g$ be defined by \eqref{eq:dual-closed-form}. Then, for every $\lambda \ge 0$ for which differentiation
under the expectation is justified,
\begin{equation}
g'(\lambda)
=
\tau
-
\mathbb{E}_{x \sim D_x}
\mathbb{E}_{y \sim \pi_\lambda^*(\cdot\mid x)}[c(x,y)].
\label{eq:dual-gradient}
\end{equation}
Moreover,
\begin{equation}
g''(\lambda)
=
\frac{1}{\beta}
\mathbb{E}_{x \sim D_x}
\operatorname{Var}_{y \sim \pi_\lambda^*(\cdot\mid x)}\!\big(c(x,y)\big)
\ge 0.
\label{eq:dual-hessian}
\end{equation}
Hence, $g$ is convex on $\mathbb{R}_+$.
\end{corollary}

\begin{proof}
Let
\[
A_x(\lambda)
:=
\beta \log
\mathbb{E}_{y \sim \pi_{\mathrm{ref}}(\cdot \mid x)}
\left[
\exp\!\left(\frac{r(x,y)-\lambda c(x,y)}{\beta}\right)
\right].
\]
Then $g(\lambda)=\mathbb{E}_{x\sim D_x}[A_x(\lambda)] + \lambda\tau$.
Differentiating gives
\[
A_x'(\lambda)
=
-\mathbb{E}_{y \sim \pi_\lambda^*(\cdot\mid x)}[c(x,y)],
\]
which implies \eqref{eq:dual-gradient}. Differentiating once more yields
\[
A_x''(\lambda)
=
\frac{1}{\beta}
\operatorname{Var}_{y \sim \pi_\lambda^*(\cdot\mid x)}\!\big(c(x,y)\big),
\]
and \eqref{eq:dual-hessian} follows by averaging over $x$.
\end{proof}

\begin{remark}
Proposition \ref{prop:primal-safe} is exact when the optimization in \eqref{eq:primal-safe} ranges over all conditional
distributions $\pi(\cdot\mid x)$ absolutely continuous with respect to $\pi_{\mathrm{ref}}(\cdot\mid x)$.
If one instead restricts to a parameterized nonconvex class $\{\pi_\theta : \theta \in \Theta\}$, then
\eqref{eq:dual-closed-form} need not coincide with the exact dual function of the restricted problem.
In that case, \eqref{eq:dual-closed-form} should be interpreted as the dual of the unrestricted problem,
and therefore as an upper bound (or relaxation) of the restricted primal objective.
\end{remark}

%%%%%%%%%%%%%%%%%%
