# Supplementary material for: Safe Inference-Time Alignment via Lagrangian Reward Augmentation
Source: arXiv:2607.02781 source file (2026-11-25)
Supplement: Supplementary file 2 [file appendix_dual_conc.tex]

\section{A finite-sample high-probability guarantee for estimating the dual variable}

We fix a compact search interval $I := [0,\Lambda] \subset \mathbb{R}_{+}$ and consider the population dual objective
\[
g(\lambda)
:=
\mathbb{E}\!\left[\phi(X,\lambda)\right],
\qquad
\phi(x,\lambda)
:=
\beta \log Z_x(\lambda) + \lambda \tau,
\]
where
\[
Z_x(\lambda)
:=
\mathbb{E}_{Y \sim \pi_{\mathrm{ref}}(\cdot \mid x)}
\exp\!\left(\frac{r(x,Y)-\lambda c(x,Y)}{\beta}\right).
\]
Given iid prompts $X_1,\dots,X_N$, the empirical objective is
\[
\hat g_N(\lambda)
:=
\frac{1}{N}\sum_{i=1}^N \phi(X_i,\lambda).
\]
We denote by
\[
\lambda^\star := \arg\min_{\lambda \in I} g(\lambda),
\qquad
\hat\lambda_N \in \arg\min_{\lambda \in I} \hat g_N(\lambda)
\]
the population and empirical minimizers, respectively.

We make the following assumptions.
\begin{assumption}\label{assump:dual-estimation}
The following hold.
\begin{enumerate}
    \item \(X_1,\dots,X_N\) are iid.
    \item The inner expectation defining \(Z_x(\lambda)\) is computed exactly. \label{assump:de-inner}
    \item The cost is uniformly bounded: there exists \(C>0\) such that
    \[
    0\le c(x,y)\le C
    \qquad\text{for all }(x,y).
    \]
    \item The threshold satisfies \(0\le \tau\le C\).
    \item The population objective \(g\) has a unique minimizer \(\lambda^\star\in(0,\Lambda)\).
    \item \(g\) is twice continuously differentiable on \([0,\Lambda]\), and there exists \(\mu>0\) such that
    \[
    g''(\lambda)\ge \mu
    \qquad\text{for all }\lambda\in[0,\Lambda].
    \]
\end{enumerate}
\end{assumption}

Note that the assumption that the inner expectation is computed exactly is a simplifying one, which allows us to focus on the statistical error from outer sampling without having to deal with the additional technicalities of inner estimation error. When the inner expectation is estimated from samples, one obtains the same type of guarantee with an additional error term depending on the number of sampled responses per prompt. The last assumption follows from the strong convexity of the dual objective.

% Let $X_1,\dots,X_N$ be iid draws from the prompt distribution; this isolates the statistical error due to outer sampling. For simplicity, we assume that the inner expectation in $Z_x(\lambda)$ is computed exactly, so that the only source of randomness is the calibration batch. This allows us to focus on the statistical error from outer sampling without having to deal with the additional technicalities of inner estimation error. When the inner expectation is estimated from samples, one obtains the same type of guarantee with an additional error term depending on the number of sampled responses per prompt.
% We assume that the cost is bounded as $0 \le c(x,y) \le C$ for all $(x,y)$, which is natural when the cost model is normalized or clipped; we also assume $0 \le \tau \le C$, so that the constraint level lives on the same scale. We also assume that the minimizer $\lambda^\star$ lies in the interior of $I$.
% % Fourth, $g$ has a unique minimizer $\lambda^\star \in (0,\Lambda)$; this ensures identifiability and avoids boundary effects. 
% Finally, recall that $g$ is strongly convex, i.e. it is twice differentiable on $[0,\Lambda]$ and there exists $\mu > 0$ such that
% \[
% g''(\lambda) \ge \mu
% \qquad
% \text{for all } \lambda \in [0,\Lambda].
% \]
% This ensures that the population minimizer $\lambda^\star$ is unique.

\begin{theorem}
Let
\[
m := \min\{\lambda^\star,\ \Lambda-\lambda^\star\}
\]
and
\[
\varepsilon_N(\delta)
:=
C \sqrt{\frac{2\log(2(N+1)/\delta)}{N}}
+
\frac{C^2 \Lambda}{4\beta N}.
\]
If $\varepsilon_N(\delta) < \mu m$, then under Assumption~\ref{assump:dual-estimation}
\[
\mathbb{P}\!\left(
|\hat\lambda_N - \lambda^\star|
\le
\frac{\varepsilon_N(\delta)}{\mu}
\right)
\ge 1-\delta.
\]
\end{theorem}

\begin{proof}
We proceed in four steps.

\paragraph{Step 1: derivatives of the sample loss.}
For each $(x,\lambda)$, define the tilted distribution
\[
\pi_\lambda^\star(y \mid x)
:=
\frac{
\pi_{\mathrm{ref}}(y \mid x)
\exp\!\left(\frac{r(x,y)-\lambda c(x,y)}{\beta}\right)
}{
Z_x(\lambda)
}
\]
and the corresponding expected cost
\[
\bar c_\lambda(x)
:=
\mathbb{E}_{Y \sim \pi_\lambda^\star(\cdot \mid x)}[c(x,Y)].
\]
We claim that
\[
\phi'(x,\lambda) = \tau - \bar c_\lambda(x)
\]
and
\[
\phi''(x,\lambda)
=
\frac{1}{\beta}
\operatorname{Var}_{Y \sim \pi_\lambda^\star(\cdot \mid x)}\!\big(c(x,Y)\big).
\]

Indeed, differentiating $Z_x(\lambda)$ gives
\[
Z_x'(\lambda)
=
\mathbb{E}_{Y \sim \pi_{\mathrm{ref}}(\cdot \mid x)}
\left[
-\frac{c(x,Y)}{\beta}
\exp\!\left(\frac{r(x,Y)-\lambda c(x,Y)}{\beta}\right)
\right].
\]
Therefore,
\begin{align*}
\phi'(x,\lambda)
&=
\beta \frac{Z_x'(\lambda)}{Z_x(\lambda)} + \tau \\
&=
-\frac{
\mathbb{E}_{Y \sim \pi_{\mathrm{ref}}(\cdot \mid x)}
\left[
c(x,Y)\exp\!\left(\frac{r(x,Y)-\lambda c(x,Y)}{\beta}\right)
\right]
}{
\mathbb{E}_{Y \sim \pi_{\mathrm{ref}}(\cdot \mid x)}
\left[
\exp\!\left(\frac{r(x,Y)-\lambda c(x,Y)}{\beta}\right)
\right]
}
+ \tau \\
&=
\tau - \bar c_\lambda(x).
\end{align*}
Differentiating once more yields
\[
\frac{d}{d\lambda}\bar c_\lambda(x)
=
-\frac{1}{\beta}
\operatorname{Var}_{Y \sim \pi_\lambda^\star(\cdot \mid x)}\!\big(c(x,Y)\big),
\]
and hence
\[
\phi''(x,\lambda)
=
-\frac{d}{d\lambda}\bar c_\lambda(x)
=
\frac{1}{\beta}
\operatorname{Var}_{Y \sim \pi_\lambda^\star(\cdot \mid x)}\!\big(c(x,Y)\big).
\]

In particular,
\[
g'(\lambda) = \mathbb{E}[\phi'(X,\lambda)],
\qquad
\hat g_N'(\lambda)
=
\frac{1}{N}\sum_{i=1}^N \phi'(X_i,\lambda).
\]
Moreover, since $0 \le c(x,y) \le C$, any random variable supported on $[0,C]$ has variance at most $C^2/4$. Hence
\[
0 \le \phi''(x,\lambda) \le \frac{C^2}{4\beta},
\]
which implies
\[
0 \le g''(\lambda) \le \frac{C^2}{4\beta}
\qquad
\text{for all } \lambda \in [0,\Lambda].
\]
Therefore $g'$ is Lipschitz on $[0,\Lambda]$ with Lipschitz constant
\[
L := \frac{C^2}{4\beta}.
\]

\paragraph{Step 2: concentration on a finite grid.}
Fix an integer $M \ge 1$, and define the grid
\[
\lambda_j := \frac{j\Lambda}{M},
\qquad
j = 0,1,\dots,M,
\]
with spacing
\[
\Delta := \frac{\Lambda}{M}.
\]
For each grid point $\lambda_j$, define
\[
Z_i^{(j)} := \phi'(X_i,\lambda_j).
\]
Since $0 \le \bar c_{\lambda_j}(x) \le C$ and $0 \le \tau \le C$, we have
\[
-C \le Z_i^{(j)} \le C
\qquad
\text{almost surely.}
\]
Also, for each fixed $j$, the variables $Z_1^{(j)},\dots,Z_N^{(j)}$ are iid. Since
\[
\hat g_N'(\lambda_j) = \frac{1}{N}\sum_{i=1}^N Z_i^{(j)},
\qquad
g'(\lambda_j) = \mathbb{E}[Z_i^{(j)}],
\]
Hoeffding's inequality gives, for every $t>0$,
\[
\mathbb{P}\!\left(
\left|
\hat g_N'(\lambda_j)-g'(\lambda_j)
\right| > t
\right)
\le
2\exp\!\left(-\frac{Nt^2}{2C^2}\right).
\]
Applying the union bound over the $M+1$ grid points yields
\[
\mathbb{P}\!\left(
\max_{0 \le j \le M}
\left|
\hat g_N'(\lambda_j)-g'(\lambda_j)
\right| > t
\right)
\le
2(M+1)\exp\!\left(-\frac{Nt^2}{2C^2}\right).
\]
Now set
\[
t_{N,M}(\delta)
:=
C\sqrt{\frac{2\log(2(M+1)/\delta)}{N}}.
\]
Then
\[
\mathbb{P}\!\left(
\max_{0 \le j \le M}
\left|
\hat g_N'(\lambda_j)-g'(\lambda_j)
\right|
\le
t_{N,M}(\delta)
\right)
\ge 1-\delta.
\]
Let $\mathcal E_{N,M}(\delta)$ denote this event.

\paragraph{Step 3: from grid control to uniform derivative control.}
We show that on $\mathcal E_{N,M}(\delta)$,
\[
\sup_{\lambda \in [0,\Lambda]}
\left|
\hat g_N'(\lambda)-g'(\lambda)
\right|
\le
t_{N,M}(\delta) + L\Delta.
\]

Fix any $\lambda \in [0,\Lambda]$, and choose $j \in \{0,\dots,M-1\}$ such that
\[
\lambda \in [\lambda_j,\lambda_{j+1}].
\]
Since $\hat g_N$ is convex and differentiable, its derivative $\hat g_N'$ is monotone nondecreasing. Therefore,
\[
\hat g_N'(\lambda_j)
\le
\hat g_N'(\lambda)
\le
\hat g_N'(\lambda_{j+1}).
\]

For the upper bound, we write
\begin{align*}
\hat g_N'(\lambda)-g'(\lambda)
&\le
\hat g_N'(\lambda_{j+1})-g'(\lambda) \\
&=
\bigl(\hat g_N'(\lambda_{j+1})-g'(\lambda_{j+1})\bigr)
+
\bigl(g'(\lambda_{j+1})-g'(\lambda)\bigr).
\end{align*}
On $\mathcal E_{N,M}(\delta)$, the first term is at most $t_{N,M}(\delta)$. Since $g'$ is $L$-Lipschitz and $|\lambda_{j+1}-\lambda| \le \Delta$, the second term is at most $L\Delta$. Hence
\[
\hat g_N'(\lambda)-g'(\lambda)
\le
t_{N,M}(\delta)+L\Delta.
\]

For the lower bound, similarly,
\begin{align*}
\hat g_N'(\lambda)-g'(\lambda)
&\ge
\hat g_N'(\lambda_j)-g'(\lambda) \\
&=
\bigl(\hat g_N'(\lambda_j)-g'(\lambda_j)\bigr)
+
\bigl(g'(\lambda_j)-g'(\lambda)\bigr),
\end{align*}
and therefore, on $\mathcal E_{N,M}(\delta)$,
\[
\hat g_N'(\lambda)-g'(\lambda)
\ge
-\,t_{N,M}(\delta)-L\Delta.
\]
Combining the two bounds gives
\[
\left|
\hat g_N'(\lambda)-g'(\lambda)
\right|
\le
t_{N,M}(\delta)+L\Delta.
\]
Since $\lambda$ was arbitrary,
\[
\sup_{\lambda \in [0,\Lambda]}
\left|
\hat g_N'(\lambda)-g'(\lambda)
\right|
\le
t_{N,M}(\delta)+L\Delta.
\]

\paragraph{Step 4: localization of the empirical minimizer.}
Assume now that
\[
t_{N,M}(\delta)+L\Delta < \mu m,
\qquad
m := \min\{\lambda^\star,\ \Lambda-\lambda^\star\}.
\]
Since $\lambda^\star$ is the unique minimizer of $g$ on $[0,\Lambda]$ and $g$ is differentiable, we have
\[
g'(\lambda^\star)=0.
\]
Moreover, because $g''(\lambda)\ge \mu$ for all $\lambda \in [0,\Lambda]$, for every $\lambda \ge \lambda^\star$,
\[
g'(\lambda)
=
\int_{\lambda^\star}^{\lambda} g''(u)\,du
\ge
\mu(\lambda-\lambda^\star),
\]
and for every $\lambda \le \lambda^\star$,
\[
g'(\lambda)
=
-\int_{\lambda}^{\lambda^\star} g''(u)\,du
\le
-\mu(\lambda^\star-\lambda).
\]

Set
\[
\varepsilon := t_{N,M}(\delta)+L\Delta.
\]
If $\lambda \ge \lambda^\star + \varepsilon/\mu$, then
\[
g'(\lambda)\ge \varepsilon,
\]
and therefore, on $\mathcal E_{N,M}(\delta)$,
\[
\hat g_N'(\lambda)
\ge
g'(\lambda)-\varepsilon
\ge 0.
\]
Likewise, if $\lambda \le \lambda^\star - \varepsilon/\mu$, then
\[
g'(\lambda)\le -\varepsilon,
\]
so on $\mathcal E_{N,M}(\delta)$,
\[
\hat g_N'(\lambda)
\le
g'(\lambda)+\varepsilon
\le 0.
\]

Because $\varepsilon < \mu m$, the interval
\[
\left[
\lambda^\star-\frac{\varepsilon}{\mu},
\,
\lambda^\star+\frac{\varepsilon}{\mu}
\right]
\]
lies strictly inside $[0,\Lambda]$. Since $\hat g_N$ is convex, the sign information on $\hat g_N'$ implies that $\hat g_N$ is nonincreasing to the left of this interval and nondecreasing to the right of it. Hence every minimizer of $\hat g_N$ over $[0,\Lambda]$ must lie inside the interval. In particular,
\[
|\hat\lambda_N-\lambda^\star|
\le
\frac{\varepsilon}{\mu}
=
\frac{t_{N,M}(\delta)+L\Delta}{\mu}
\]
on the event $\mathcal E_{N,M}(\delta)$.

Therefore,
\[
\mathbb{P}\!\left(
|\hat\lambda_N-\lambda^\star|
\le
\frac{t_{N,M}(\delta)+L\Delta}{\mu}
\right)
\ge
1-\delta.
\]

% \paragraph{Step 5: substitute $M=N$.}
We now choose the grid size deterministically as $M=N$. Then
\[
\Delta = \frac{\Lambda}{N},
\qquad
t_{N,N}(\delta)
=
C\sqrt{\frac{2\log(2(N+1)/\delta)}{N}},
\]
and therefore
\[
t_{N,N}(\delta)+L\Delta
=
C\sqrt{\frac{2\log(2(N+1)/\delta)}{N}}
+
\frac{C^2}{4\beta}\frac{\Lambda}{N}
=
\varepsilon_N(\delta).
\]
Thus, provided $\varepsilon_N(\delta) < \mu m$, we conclude that
\[
\mathbb{P}\!\left(
|\hat\lambda_N-\lambda^\star|
\le
\frac{\varepsilon_N(\delta)}{\mu}
\right)
\ge
1-\delta,
\]
as claimed.
\end{proof}
